# Supplementary material for: Exploiting Opportunistic Physical Design in Large-scale Data Analytics
Source: arXiv:1303.6609 source file (2013-12-10)
Supplement: Supplementary file 1 [file appendix.pdf]

## A Longer versions of Proofs

**Theorem 1** *BFREWRITE finds the optimal rewrite  $r^*$  of  $W$  and is work-efficient.*

**Proof** To ensure correctness, BFREWRITE must not terminate before finding  $r^*$ . Correctness requires that we show the algorithm examines every candidate view with OPTCOST less than or equal to  $\text{COST}(r^*)$ . To ensure work-efficiency, BFREWRITE should not examine any extra views that cannot be included in  $r^*$ . Work-efficiency requires that we show the algorithm must not examine any candidate view with OPTCOST greater than  $\text{COST}(r^*)$ . We first prove these two properties of BFREWRITE for a query  $W$  containing a single target, then extend these results to the case when  $W$  contains  $n$  targets.

For  $W$  with a single target (i.e.,  $n = 1$ ), proof by contradiction proceeds as follows. Consider two different rewrites  $r$  and  $r^*$  such that  $r^*$  is the optimal rewrite and  $\text{COST}(r^*) < \text{COST}(r)$ . Assume a candidate view  $v^*$  produces the optimal rewrite  $r^*$ . Assume another candidate view  $v$  produces the rewrite  $r$ . Suppose that BFREWRITE examines  $v$ , sets  $\text{BESTPLANCOST}_n$  to  $\text{COST}(r)$ , and then terminates before examining  $v^*$ . Hence BFREWRITE incorrectly reports  $r$  as the optimal rewrite even though  $\text{COST}(r^*) < \text{COST}(r)$ . Because BFREWRITE examines candidate views by increasing OPTCOST, then since  $v$  was examined before  $v^*$ , it must have been the case that  $\text{OPTCOST}(v) < \text{OPTCOST}(v^*)$ . By design, BFREWRITE will continue until all candidate views whose OPTCOST is less than or equal to  $\text{BESTPLANCOST}_n$  have been found. Given the lower bound property of OPTCOST with respect to COST, we have that:

$$\text{OPTCOST}(v) < \text{OPTCOST}(v^*) \leq \text{COST}(r^*) < \text{COST}(r) = \text{BESTPLANCOST}_n.$$

From the above inequality, it is clear that the algorithm must have examined  $v^*$  (and consequently found  $r^*$ ) before terminating. This results in a contradiction since we assumed earlier that BFREWRITE terminated before examining  $v^*$ .

We can similarly prove work-efficiency by contradiction as follows. Assume that  $\text{OPTCOST}(v) > \text{COST}(r^*)$  and as above the algorithm examines  $v$  before  $v^*$ . This results in the following inequality.

$$\text{COST}(r^*) < \text{OPTCOST}(v) \leq \text{COST}(r) = \text{BESTPLANCOST}_n < \text{OPTCOST}(v^*).$$

The results in a contradiction since  $\text{COST}(r^*)$  cannot be less than  $\text{OPTCOST}(v^*)$ , based on the lower-bound property of OPTCOST.

Now we extend this result to  $W$  with multiple targets,  $n > 1$ . It is sufficient to show that the BFREWRITE algorithm works by reducing  $n$  individual search problems into a single global search problem that finds the optimal rewrite for the target  $W_n$ . Recall that BFREWRITE instantiates a priority queue  $PQ$  at each of the  $n$  targets in the plan, where the candidate views at each  $PQ$  are ordered by increasing OPTCOST. Next we show that the search process degenerates these  $n$  PQs into a single virtual global  $PQ$  whose elements are potential rewrites of  $W_n$ , ordered by their increasing OPTCOST. Recall that every invocation of FINDNEXTMINTARGET identifies the next best target to refine out of all targets in  $W$ . It composes the lowest cost potential rewrite for  $W_n$  by recursively visiting each target  $W_i$  and selecting the cheaper among either the candidate view at the front of the  $PQ$  for  $W_i$  or the current best known rewrite for  $W_i$ . Thus this recursive procedure identifies the current lowest cost potential rewrite of  $W_n$ , in effect gradually exploring the space of potential rewrites of  $W_n$  by their increasing OPTCOST. This creates a virtual global  $PQ$  whose elements are potential rewrites of  $W_n$  and is ordered by their OPTCOST.

For example, in Figure 6, note that the first potential rewrite for  $W_n$  is composed of  $a, c, n_3$  with an OPTCOST of 5, while the next potential rewrite of  $W_n$  is composed of  $b$  with an OPTCOST of 6. Furthermore, notice that the rewrite produced by  $a, c, n_3$  has a cost of 10, which is always greater than or equal to its corresponding OPTCOST due to the lower-bound property. We have now reduced  $n$  priority queues of candidate views ordered by OPTCOST to a single global priority queue of potential rewrites of  $W_n$  ordered by OPTCOST. This completes the proof since we already showed above that BFREWRITE with a single  $PQ$  ordered by OPTCOST will find the optimal rewrite and is work-efficient.

**Theorem 2** *The OPTCOST of every candidate view in  $M$  that is not in  $Seen$  is greater than or equal to the OPTCOST of  $v$ .*

**Proof** The proof sketch is as follows. The theorem is trivially true for  $v \in V$  as all candidate views in  $M$  cannot be in  $Seen$  and have OPTCOST greater than  $v$ . If  $v \notin V$ , it is sufficient to point out that all constituent views of  $v$  are already in  $Seen$  since they must have had OPTCOST lesser or equal to  $v$ . Hence all candidate views in  $M$  with OPTCOST smaller than  $v$  are already in  $Seen$ , and those with OPTCOST greater than  $v$  will be added to  $PQ$  if they are not already in  $PQ$ .

# B Annotations for Piggybank and DataFu UDFs

The required info for the UDF model annotations were inferred from the Javadocs in less than a day, or about 10 minutes per UDF. This is a one-time effort per UDF.

Piggybank: <http://pig.apache.org/docs/r0.11.0/api/overview-summary.html>

| Classpath |                                                                        | UDF_Usage_Example                        | input                 | output                 | model_input              | model_output           | derived attrs | derived attrs signature                                  |
|-----------|------------------------------------------------------------------------|------------------------------------------|-----------------------|------------------------|--------------------------|------------------------|---------------|----------------------------------------------------------|
| Piggybank | org.apache.pig.piggybank.evaluation.ExtremalTupleByNthField            | ExtremalTupleByNthField(bag1,"4", "max") | bag1, fieldnum, order | extrema                | A={bag1}; F=x, K=y       | A={extrema} F=x; K=y   | extrema       | extrema={model_input; UDF_name; ARGS = fieldnum,order}   |
| Piggybank | org.apache.pig.piggybank.evaluation.MaxTupleBy1stField                 | MaxTupleBy1stField(bag1)                 | bag1                  | extrema                | A={bag1}; F=x, K=y       | A={extrema} F=x; K=y   | extrema       | extrema={model_input; UDF_name}                          |
| Piggybank | org.apache.pig.piggybank.evaluation.datetime.DiffDate                  | DiffDate(date1,date2)                    | date1, date2          | date1, date2, datediff | A={date1,date2}; F=x;K=y | A={datediff}; F=x;K=y  | datediff      | datediff={model_input; UDF_name}                         |
| Piggybank | org.apache.pig.piggybank.evaluation.datetime.convert.CustomFormatToISO | CustomFormatToISO(date, "MM-dd-YYYY")    | date, desiredformat   | date, customdate       | A={date};F=x;K=y         | A={customdate};F=x;K=y | customdate    | customdate={model_input; UDF_name; ARGS = desiredformat} |
| Piggybank | org.apache.pig.piggybank.evaluation.datetime.diff.ISODaysBetween       | ISODaysBetween(date1,date2)              | date1, date2          | date1, date2, datediff | A={date1,date2}; F=x;K=y | A={datediff}; F=x;K=y  | datediff      | datediff={model_input; UDF_name}                         |

|           |                                                                                |                                                                                         |                                            |                              |                                        |                                                             |                    |                                                                             |
|-----------|--------------------------------------------------------------------------------|-----------------------------------------------------------------------------------------|--------------------------------------------|------------------------------|----------------------------------------|-------------------------------------------------------------|--------------------|-----------------------------------------------------------------------------|
| Piggybank | org.apache.pig.piggybank.evaluation.datetime.truncate.ISOToDay                 | ISOToDay(date1)                                                                         | date1                                      | date1,day                    | A={date1};F=x;K=y                      | A={day};F=x;K=y                                             | day                | day={model_input; UDF_name}                                                 |
| Piggybank | org.apache.pig.piggybank.evaluation.decode.Bin                                 | Bin(Salary, "\$50K--\$100k", "Engineer", "\$100K--\$200K", "Manager")                   | Salary, value1, label1, value2, label2 ... | Salary, JobTitle             | A={Salary};F=x;K=y                     | A={Salary,JobTitle};F=x;K=y                                 | JobTitle           | JobTitle={model_input; UDF_name; ARGS = value1, label1, value2, label2 ...} |
| Piggybank | org.apache.pig.piggybank.evaluation.decode.BinCond                             | BinCond(Salary, "Salary <= \$100k", "Engineer", "\$100K<= Salary <= \$200K", "Manager") | Salary, value1, label1, value2, label2 ... | Salary, JobTitle             | A={Salary};F=x;K=y                     | A={Salary,JobTitle};F=x;K=y                                 | JobTitle           | JobTitle={model_input; UDF_name; ARGS = value1, label1, value2, label2 ...} |
| Piggybank | org.apache.pig.piggybank.evaluation.decode.Decode                              | Decode(Salary, "\$100k", "Engineer", "\$200K", "Manager")                               | Salary, value1, label1, value2, label2 ... | Salary, JobTitle             | A={Salary};F=x;K=y                     | A={Salary,JobTitle};F=x;K=y                                 | JobTitle           | JobTitle={model_input; UDF_name; ARGS = value1, label1, value2, label2 ...} |
| Piggybank | org.apache.pig.piggybank.evaluation.math                                       | We skip these since these are standard math functions.                                  |                                            |                              |                                        |                                                             |                    |                                                                             |
| Piggybank | org.apache.pig.piggybank.evaluation.stats.COR;org.apache.pig.builtin.COR       | COR.computeAll(OilSupply, GasPrice)                                                     | OilSupply,GasPrice                         | OilSupply,GasPrice, CorScore | A={OilSupply,GasPrice};F=x;K=y         | A={OilSupply,GasPrice, CorScore};F=x;K={OilSupply,GasPrice} | CorScore           | CorScore={model_input; UDF_name}                                            |
| Piggybank | org.apache.pig.piggybank.evaluation.stats.COV;org.apache.pig.builtin.COV       | COV.computeAll(OilSupply, GasPrice)                                                     | OilSupply,GasPrice                         | OilSupply,GasPrice, CovScore | A={OilSupply,GasPrice};F=x;K=y         | A={OilSupply,GasPrice, CovScore};F=x;K={OilSupply,GasPrice} | CovScore           | CovScore={model_input; UDF_name}                                            |
| Piggybank | org.apache.pig.piggybank.evaluation.util.SearchQuery                           | SearchQuery(url_string)                                                                 | UrlString                                  | QueryString                  | A={UrlString};F=x;K=Y                  | A={QueryString};F=x;K=y                                     | QueryString        | QueryString={model_input; UDF_name}                                         |
| Piggybank | org.apache.pig.piggybank.evaluation.util.apachelogparser.DateExtractor         | DateExtractor(dayTime, "yyyy-MM", "GMT")                                                | dayTime, outdatestring, tz                 | customdate                   | A={dayTime, outdatestring, tz};F=x;K=y | A={customdate};F=x;K=y                                      | customdate         | customdate={model_input; UDF_name; ARGS=outdatestring,tz}                   |
| Piggybank | org.apache.pig.piggybank.evaluation.util.apachelogparser.HostExtractor         | HostExtractor(referer_url)                                                              | referer_url                                | host_url                     | A={referer_url};F=x;K=y                | A={host_url};F=x;K=y                                        | host_url           | host_url={model_input; UDF_name}                                            |
| Piggybank | org.apache.pig.piggybank.evaluation.util.apachelogparser.SearchEngineExtractor | SearchEngineExtractor(referer_url)                                                      | referer_url                                | search_engine_name           | A={referer_url};F=x;K=y                | A={search_engine_name};F=x;K=y                              | search_engine_name | search_engine_name={model_input; UDF_name}                                  |
| Piggybank | org.apache.pig.piggybank.evaluation.util.apachelogparser.SearchTermExtractor   | SearchTermExtractor(referer_url)                                                        | referer_url                                | search_terms                 | A={referer_url};F=x;K=y                | A={search_terms};F=x;K=y                                    | search_terms       | search_terms={model_input; UDF_name}                                        |
| Piggybank | org.apache.pig.piggybank.storage                                               | We skip these since they are custom file formatting functions.                          |                                            |                              |                                        |                                                             |                    |                                                                             |

| DataFu: <a href="http://linkedin.github.io/datafu/docs/current/">http://linkedin.github.io/datafu/docs/current/</a> |                                      |                                       |                         |                |                       |                                                                    |                         |                                                                                                                                       |
|---------------------------------------------------------------------------------------------------------------------|--------------------------------------|---------------------------------------|-------------------------|----------------|-----------------------|--------------------------------------------------------------------|-------------------------|---------------------------------------------------------------------------------------------------------------------------------------|
| Classpath                                                                                                           | UDF_Usage_Example                    | input                                 | output                  | model_input    | model_output          | derived attrs                                                      | derived attrs signature |                                                                                                                                       |
| DataFu                                                                                                              | datafu.pig.bags.AppendToBag          | AppendToBag(bag1, "{1,2,3,4}")        | bag1, tup1              | bag2           | A={bag1};F=x;K=y      | A={bag2};F=x;K=y                                                   | bag2                    | bag2={model_input; UDF_name; ARGS=tup1}                                                                                               |
| DataFu                                                                                                              | datafu.pig.bags.BagConcat            | BagConcat(bag1,bag2)                  | bag1,bag2               | bag3           | A={bag1,bag2};F=x;K=y | A={bag1,bag2};F=x;K=y                                              | bag3                    | bag3={model_input; UDF_name}                                                                                                          |
| DataFu                                                                                                              | datafu.pig.bags.BagGroup             | BagGroup(bag1, "4")                   | bag1,keypos             | key,bag2       | A={bag1};F=x;K=y      | A={key,bag2};F=x;K={key}                                           | key,bag2                | key={model_input;UDF_name, ARGS = keypos <key>; bag2={model_input;UDF_name; ARGS = keypos<bag>}                                       |
| DataFu                                                                                                              | datafu.pig.bags.BagLeftOuterJoin     | BagLeftOuterJoin(bag1,"4", bag2, "2") | bag1,keypos,bag2,keypos | key1,key2,bag3 | A={bag1,bag2};F=x;K=y | A={key1,key2,bag3};F=x & key1==key2 or key1 is null;K={key1,key2}; | key1,key2,bag3          | key1={bag1;F=x;K=y;UDF_name,ARGS = keypos1}; key1={bag2;F=x;K=y;UDF_name, ARGS = keypos2};bag3={model_input;UDF_name; ARGS = keypos2} |
| DataFu                                                                                                              | datafu.pig.bags.BagSplit             | BagSplit(bag1, "5")                   | bag1, how               | bag2           | A={bag1};F=x;K=y      | A={bag2};F=x;K=y                                                   | bag2                    | bag2={model_input; UDF_name; ARGS = how}                                                                                              |
| DataFu                                                                                                              | datafu.pig.bags.CountEach            | CountEach(bag1)                       | bag1                    | key, count     | A={bag1};F=x;K=y      | A={key,count};F=x;K={key}                                          | key,count               | key={model_input;UDF_name,<key>; count={model_input;UDF_name; <bag>}                                                                  |
| DataFu                                                                                                              | datafu.pig.bags.DistinctBy           | DistinctBy(bag1, "4")                 | bag1,keypos             | key            | A={bag1};F=x;K=y      | A={key};F=x;K={key}                                                | key                     | key={model_input;UDF_name,ARGS=keypos}                                                                                                |
| DataFu                                                                                                              | datafu.pig.bags.EmptyBagToNull       | EmptyBagToNull(bag1)                  | bag1                    | bag2           | A={bag1};F=x;K=y      | A={bag2};F=x;K=y                                                   | bag2                    | bag2={model_input;UDF_name}                                                                                                           |
| DataFu                                                                                                              | datafu.pig.bags.EmptyBagToNullFields | EmptyBagToNullFields(bag1)            | bag1                    | bag2           | A={bag1};F=x;K=y      | A={bag2};F=x;K=y                                                   | bag2                    | bag2={model_input;UDF_name}                                                                                                           |
| DataFu                                                                                                              | datafu.pig.bags.Enumerate            | Enumerate(bag1)                       | bag1                    | bag2           | A={bag1};F=x;K=y      | A={bag2};F=x;K=y                                                   | bag2                    | bag2={model_input;UDF_name}                                                                                                           |

|        |                                     |                                                    |                                       |                         |                                      |                                                       |           |                                                                                                                      |
|--------|-------------------------------------|----------------------------------------------------|---------------------------------------|-------------------------|--------------------------------------|-------------------------------------------------------|-----------|----------------------------------------------------------------------------------------------------------------------|
| DataFu | datafu.pig.bags.FirstTupleFromBag   | FirstTupleFromBag(bag1)                            | bag1                                  | tuple1                  | A={bag1};F=x;K=y                     | A={tuple1};F=x;K=y                                    | tuple1    | tuple1={model_input;UDF_name}                                                                                        |
| DataFu | datafu.pig.bags.NullToEmptyBag      | NullToEmptyBag(bag1)                               | bag1                                  | bag2                    | A={bag1};F=x;K=y                     | A={bag2};F=x;K=y                                      | bag2      | bag2={model_input;UDF_name}                                                                                          |
| DataFu | datafu.pig.bags.PrependToBag        | PrependToBag(bag1, "{1,2,3,4}")                    | bag1,tuple1                           | bag2                    | A={bag1};F=x;K=y                     | A={bag2};F=x;K=y                                      | bag2      | bag2={model_input;UDF_name;ARGS=tuple1}                                                                              |
| DataFu | datafu.pig.bags.ReverseEnumerate    | ReverseEnumerate(bag1)                             | bag1                                  | bag2                    | A={bag1};F=x;K=y                     | A={bag2};F=x;K=y                                      | bag2      | bag2={model_input;UDF_name}                                                                                          |
| DataFu | datafu.pig.bags.UnorderedPairs      | UnorderedPairs(bag1)                               | bag1                                  | bag2                    | A={bag1};F=x;K=y                     | A={bag2};F=x;K=y                                      | bag2      | bag2={model_input; UDF_name}                                                                                         |
| DataFu | datafu.pig.geo.HaversineDistInMiles | HaversineDistInMiles(lat1, long1, lat2, long2)     | lat1,lon1,lat2,lon2                   | dist                    | A={lat1,lon1,lat2,lon2};F=x;K=y      | A={lat1,lon1,lat2,lon2,hdist};F=x;K=y                 | hdist     | hdist={model_input; UDF_name}                                                                                        |
| DataFu | datafu.pig.hash.MD5                 | MD5(origstring)                                    | origstring                            | origstring,md5string    | A={origstring};F=x;K=y               | A={origstring,md5string};F=x,K=y                      | md5string | md5string={model_input; UDF_name}                                                                                    |
| DataFu | datafu.pig.linkanalysis.PageRank    | PageRank(source,edges)                             | source, edges                         | source,rank             | A={source,edges};F=x;K=y             | A={source,rank};F=x;K=source                          | rank      | rank={model_input; UDF_name}                                                                                         |
| DataFu | datafu.pig.random.RandInt           | Cannot Model, this function is non-deterministic   |                                       |                         |                                      |                                                       |           |                                                                                                                      |
| DataFu | datafu.pig.sampling.ReservoirSample | Cannot Model, this function is non-deterministic   |                                       |                         |                                      |                                                       |           |                                                                                                                      |
| DataFu | datafu.pig.sampling.SampleByKey     | SampleByKey(bag1, "4", "0.5", "2347234")           | bag1,keypos, prob, seed               | key,bag2                | A={bag1};F=x;K=y                     | A={key,bag2};F=x & generateProb(seed) < prob;K={key}  | key,bag2  | key={model_input;UDF_name, ARGS=keypos <key>, seed, prob}; bag2={model_input;UDF_name; ARGS=keypos<bag>, seed, prob} |
| DataFu | datafu.pig.sampling.WeightedSample  | WeightedSample(bag1, "4", "3")                     | bag1, keypos, limit                   | bag2                    | A={bag1};F=x;K=y                     | A={bag2};F=x & generateProb(seed) < limit;K=y         | bag2      | bag2={model_input, UDF_name; ARGS=keypos, limit}                                                                     |
| DataFu | datafu.pig.sessions.SessionCount    | SessionCount(user_id, page_id, time, "10 minutes") | user_id, page_id, time, sessionLength | user_id, page_id, count | A={user_id, page_id, time}, F=x, K=y | A={user_id, page_id, count}; F=x; K={user_id,page_id} | count     | count={model_input; UDF_name; ARGS=sessionLength}                                                                    |
