# Supplementary material for: Exploiting Opportunistic Physical Design in Large-scale Data Analytics
Source: arXiv:1303.6609 source file (2013-12-10)
Supplement: Supplementary file 2 [file sec-appendix-new.tex]

\appendix
\section*{NEW}
The desirable property of the $\cost{}$ is that it must be cheap to compute.
Since a full query optimizer may be too expensive, we use a model of a query optimizer.
We treat this model as a black box, in this way $\RE{}$ and $\ocost{}$ can
utilize any functionality provided by the model or improvements to the model.
%For an RDBMS, a cost model such as in~\cite{x,y} could be used.
%Because we evaluate our framework in a MapReduce execution system,

Our cost model is based on the one in~\cite{Nyki2010},
which reduces a query $q$ to a set of $m$ jobs $\{J_1, \cdots, J_m\}$.
The cost of each job is expressed as a linear combination of
the cost to read the data ($C_{r}$)
the cost of sorting and copying ($C_{s}$),
the cost to transfer data ($C_{t}$).
and the cost to write the output of the job ($C_{w}$).

\begin{equation} \label{eq-cost}
\cost(q,v) = \sum_{i=1}^{m} C_{r}(J_i,v_i) +  C_{s}(J_i,v_i) +  C_{t}(J_i,v_i) +  C_{w}(J_i,v_i)
\end{equation}
where $v_1 = v$, and $v_{i}$ forms the input of $J_i$.

To keep the $\cost{}$ function inexpensive, our model does not consider re-ordering
of joins, predicate push down, or other types of optimizations involved in
group bys and udfs, but does merge sequential operations (e.g. a sequence of filters)
into the same job whenever possible.

This is a reasonable approach given that we have already committed to creating $v$,
and the $\RE{}$ explores all possible rewrites, such a cost function serves
our purposes here.

An extension to this basic cost model could consider push downs when computing the cost
to create $v$.  The requirements to including push-downs into the optimization
process would be to employ a cost model $\cost{}$ that is able to
apply all possible join orderings to creating $v$ along with applying filters
to all orders.

Appendix~\ref{appendix-pushdown} provides a proof for using $\RE{}$ and $\ocost$ with an extended
$\cost{}$ function that considers join ordering and predicate pushdowns,
while still producing a correct lower bound for $\RE{(v,q)}$.

There are 2 reasons we do not consider predicate push downs here.
First $\cost{}$ becomes much more expensive to invoke due to considering all
of the ordering options.
Second, we may not wish to push down a filter into $v$ since this could render $v$
less useful for answering future queries.
A more sophisticated algorithm could weigh the cost and benefits of different
versions of $v$ (with and without filters) given their benefit to other queries
and their added cost due to avoiding filter push downs.

\section{Proof of OptCost with push down predicates.}\label{appendix-pushdown}

A guessed to be complete view $v$ may itself contain several constituent views,
such that $v=< v_1 \bowtie v_2 \bowtie \cdots v_n>$.
Let the fix be defined as $S$, and $S'$ be a subset of $S$ containing
all filters and projects in $S$.

We now discuss the design of the $\ocost^p{}$ function that takes a view $v$ and
query $q$ that allows for predicate pushdown
into constituent views of $v$ as well as exploring different join
orderings of the constituent views.

Suppose  cost model $\cost^p{}$ is defined
as $\cost{}$ augmented to include
join orderings and pushdown predicates.
Let the input to $\cost^p{}$ be a set of views to join,
and a set of predicates to apply $S'$.
Then $\cost^p{}$ will produce a join ordering of
the constituent views including
predicate push downs to create $v'$ that
reduces the cost to create $v$.
Note that $v' \subseteq v$ as $v'$ may contain
predicates that have not yet been applied on $v$.

Let  $r^*$ represent the lowest cost rewrite produced by $\RE^p{(v,q)}$,
where $\RE^p{}$ represents
$\RE{}$ that has been been augmented to explore all join orderings
with pushdown predicates in $S'$.
The algorithm may apply as many predicates in $S'$
as possible but may not be able
to apply some due to additional constraints present
in $S$ which the $\RE^p{}$ must reconcile.
An example of such a constraint could be a filter
that can only be applied after an aggregate function.
Note that the $\ocost^p{}$ may not be able to consider such constraints
as it was only aware of the operations in $S'$.
After applying all applicable pushdowns, let $\RE^p{}$ produce $v''$.
Additionally, $S''$ is the remaining transformations in $S$ that
could not be applied and $S'' \subseteq S$.

The cost of $r^*$ is the cost to create $v''$
plus the cost to apply the remaining operators
$S''$ on $v''$, where $S'' \subseteq S$.
$\ocost^p{}$ computes the sum of
the cost to create and access $v'$ plus the cost of applying the
minimum operation in $S$ on $v'$ as the lower bound on
the cost of $r^*$.

Now we briefly show that $\ocost^p{}$ still provides
a lower bound on the cost of $r^*$.
The cost to create $v'$ is less than or equal to
cost to create $v''$ as $v'$ has
at least as many filters applied to it as $v''$.
Next, $\min(\cost(x, v'), \forall x \in S) \leq \cost(p, v'')$
where $p$ is a permutation of operations in $S''$.
Because $S'' \subseteq S$ the minimum
cost operation $op^*$ is present in $S$
but may not be in $S''$, and since $v' \subseteq v''$,
$\ocost^p{}$ is a lower-bound of $\RE^p{}$.$\qed$
