# Supplementary material for: Exploiting Opportunistic Physical Design in Large-scale Data Analytics
Source: arXiv:1303.6609 source file (2013-12-10)
Supplement: Supplementary file 3 [file sec-appendix-old.tex]

\appendix
\section*{OLD}
\section{Proof of OptCost with push down predicates.}\label{appendix-pushdown}

A guessed to be complete view $v$ may itself contain several constituent views,
such that $v=< v_1 \bowtie v_2 \bowtie \cdots v_n>$.
Let the fix be defined as $S$, and $S'$ be a subset of $S$ containing 
all filters and projects in $S$.

We now discuss the design of the $\ocost^p{}$ function that takes a view $v$ and 
query $q$ that allows for predicate pushdown 
into constituent views of $v$ as well as exploring different join 
orderings of the constituent views.

Suppose  cost model $\cost^p{}$ is defined
as $\cost{}$ augmented to include 
join orderings and pushdown predicates.
Let the input to $\cost^p{}$ be a set of views to join, 
and a set of predicates to apply $S'$.
Then $\cost^p{}$ will produce a join ordering of
the constituent views including
predicate push downs to create $v'$ that 
reduces the cost to create $v$.
Note that $v' \subseteq v$ as $v'$ may contain 
predicates that have not yet been applied on $v$.

Let  $r^*$ represent the lowest cost rewrite produced by $\RE^p{(v,q)}$,
where $\RE^p{}$ represents 
$\RE{}$ that has been been augmented to explore all join orderings 
with pushdown predicates in $S'$.
The algorithm may apply as many predicates in $S'$ 
as possible but may not be able
to apply some due to additional constraints present 
in $S$ which the $\RE^p{}$ must reconcile.
An example of such a constraint could be a filter 
that can only be applied after an aggregate function.  
Note that the $\ocost^p{}$ may not be able to consider such constraints
as it was only aware of the operations in $S'$.
After applying all applicable pushdowns, let $\RE^p{}$ produce $v''$.
Additionally, $S''$ is the remaining transformations in $S$ that
could not be applied and $S'' \subseteq S$.

The cost of $r^*$ is the cost to create $v''$ 
plus the cost to apply the remaining operators 
$S''$ on $v''$, where $S'' \subseteq S$.
$\ocost^p{}$ computes the sum of 
the cost to create and access $v'$ plus the cost of applying the 
minimum operation in $S$ on $v'$ as the lower bound on 
the cost of $r^*$.

Now we briefly show that $\ocost^p{}$ still provides 
a lower bound on the cost of $r^*$.
The cost to create $v'$ is less than or equal to 
cost to create $v''$ as $v'$ has 
at least as many filters applied to it as $v''$.  
Next, $\min(\cost(x, v'), \forall x \in S) \leq \cost(p, v'')$ 
where $p$ is a permutation of operations in $S''$.
Because $S'' \subseteq S$ the minimum 
cost operation $op^*$ is present in $S$ 
but may not be in $S''$, and since $v' \subseteq v''$,
$\ocost^p{}$ is a lower-bound of $\RE^p{}$.$\qed$
